# Supplementary material for: OMH: Structured Sparsity via Optimally Matched Hierarchy for Unsupervised Semantic Segmentation
Source: arXiv:2403.06546 source file (2024-04-05)
Supplement: Supplementary file 1 [file X_suppl.tex]

\clearpage
\setcounter{page}{1}
%\maketitlesupplementary

\section{Rationale}
\label{sec:rationale}
We provide figures about our hierarchy in the supplementary material.

\begin{figure*}[h]
\begin{tabular}{cc}
    \includegraphics[width=0.45\columnwidth]{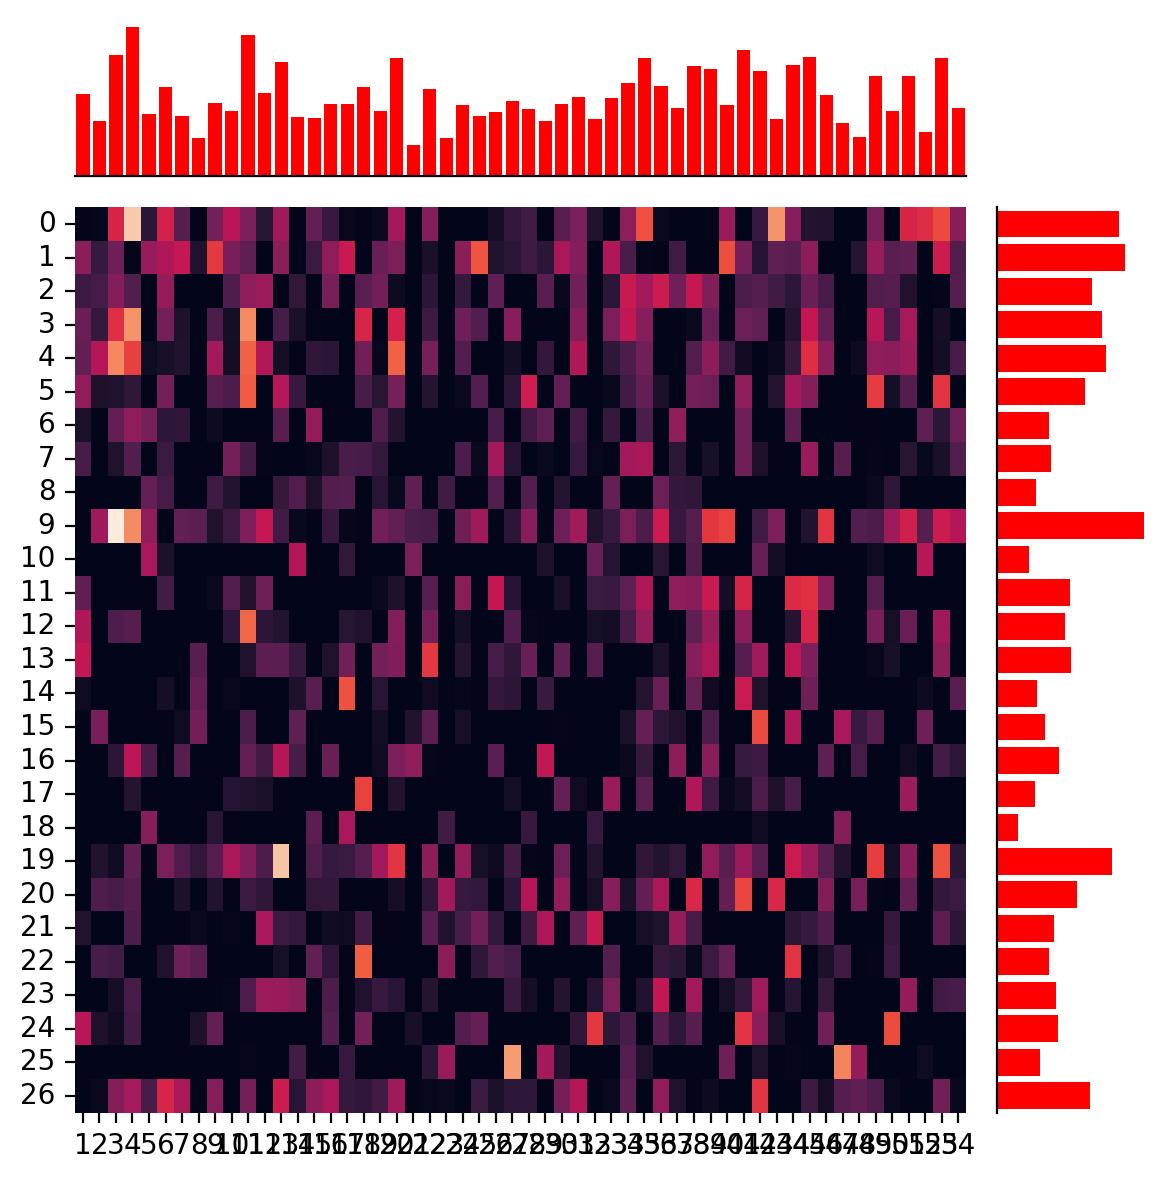} & \includegraphics[width=0.45\columnwidth]{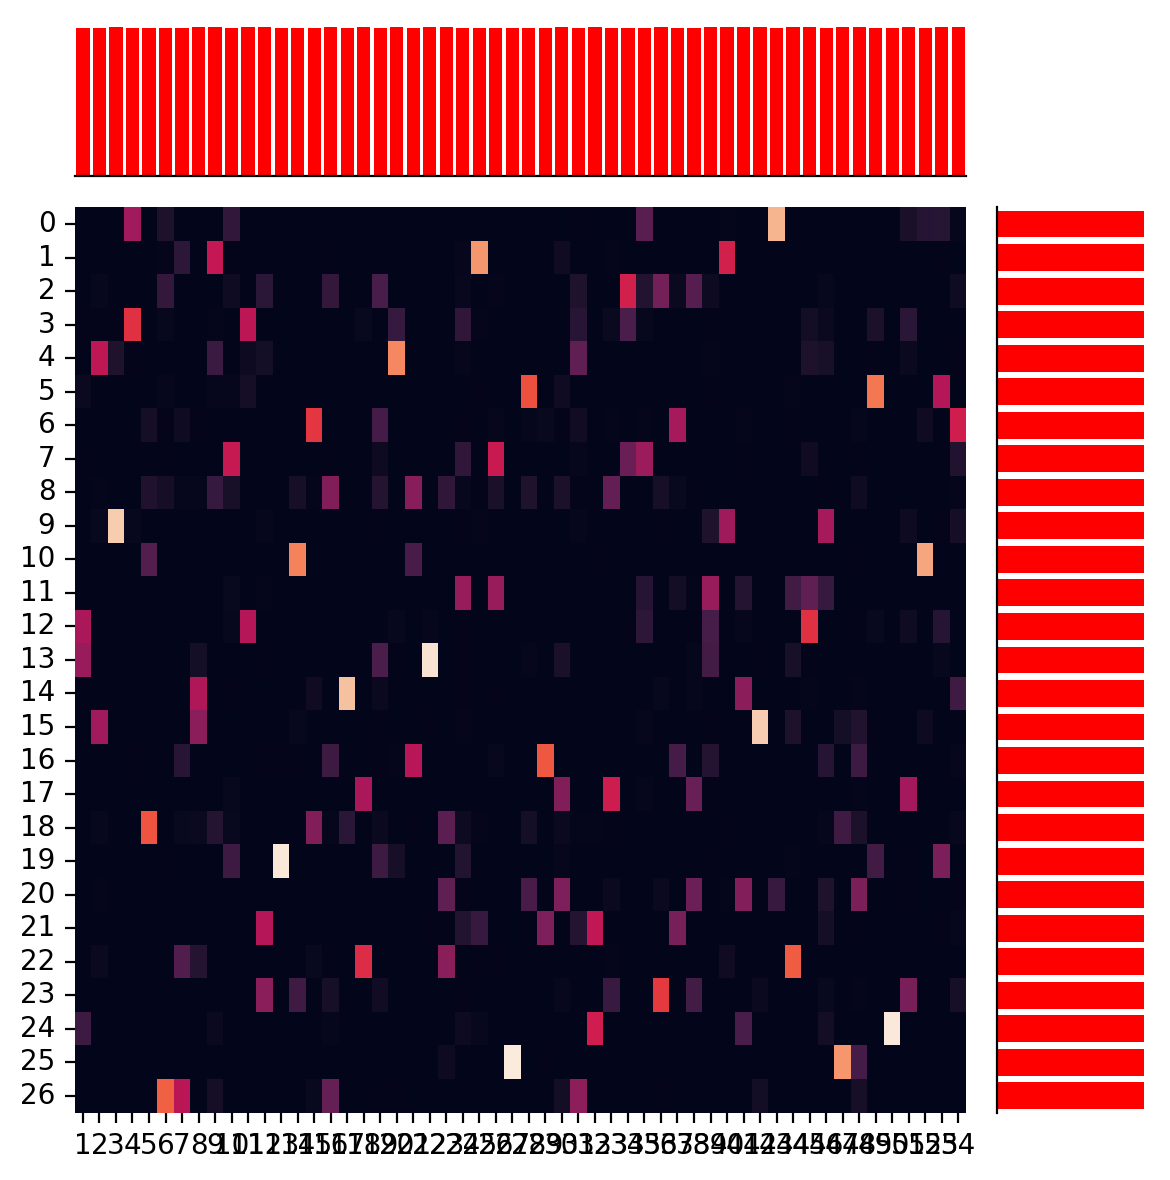} \\
     & 
\end{tabular}
\caption{{\bf Hierarchy matrix with Optimal Transport.} Optimal Transport~\cite{cuturi2013sinkhornot} leads to a sparse and balanced hierarchy. On the left, we visualize the cluster center affinities $cosim^+(\bm{H}^{(i)}, \bm{H}^{(i+1)})$ which is neither sparse (many positive similarities) nor balanced (unequal row or column sums). On the right, the optimal transportation plan $\mathbf{A}^{(i,i+1)}$ is visualized. In $\mathbf{A}^{(i,i+1)}$, two lower-level clusters are mapped to one higher-level cluster, on average, but we mostly see that some higher-level clusters are mapped to three or four lower-level clusters.}
\label{fig:hier_OT}
\end{figure*}

\begin{figure*}[h]
\begin{tabular}{cc}
    \includegraphics[width=0.45\columnwidth]{figures/fig_hier_OT.png} & \includegraphics[width=0.45\columnwidth]{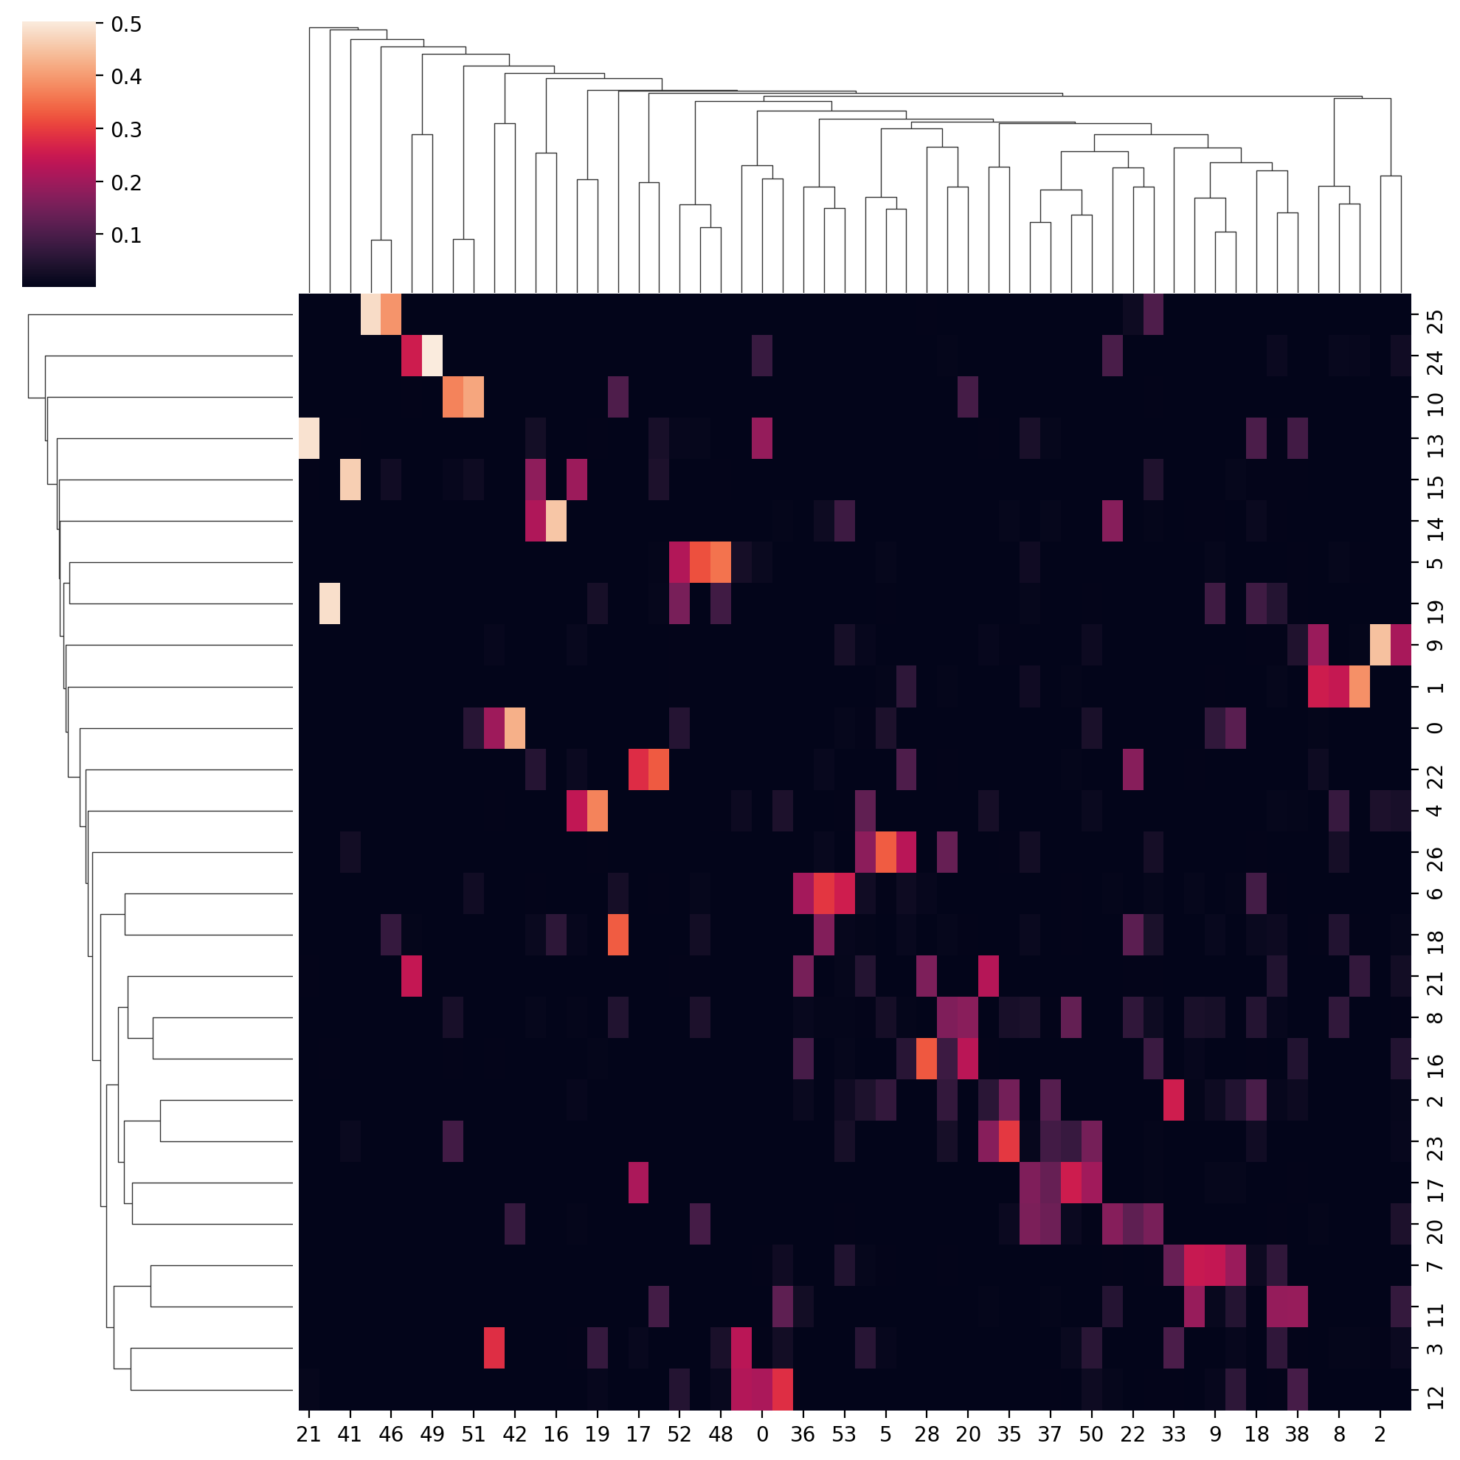} \\
     & 
\end{tabular}
\caption{{\bf Reordering the hierarchy matrix.} We also visualized a row/column permuted version of our hierarchy. In this version, similar rows and columns are closer to each other. It can be observed that this matrix imitates a one-to-two hierarchy with some relaxation.}
\label{fig:hier_OT}
\end{figure*}
